# Supplementary material for: LiDAR-EDIT: LiDAR Data Generation by Editing the Object Layouts in Real-World Scenes
Source: arXiv:2412.00592 source file (2025-05-24)
Supplement: Supplementary file 1 [file appendix.tex]

\subsection{Additional Experiment Visualizations}
Due to space limits, we only present the final shape servo results in the main text. Here, for each shape servo test case mentioned in the experiment, we provide key frames of the whole manipulation sequence (Fig. \ref{fig:additional_vis}). In addition, Fig.~\ref{fig:chamfer_plots} shows the Chamfer distance between the current object point cloud and the goal object point cloud over time when running our DeformerNet controller. 

Figure \ref{fig:init_setup} shows the experimental setup. We use the bimanual daVinci surgical robot to manipulate a soft box object which mimics human tissue. The left arm grasps one end of the object and holds it in place, while the right arm deforms the object into a desired shape.
\begin{figure}[ht!]
    \centering
    \includegraphics[scale=0.3]{figures/setup.png}
    \caption{Experimental setup of the two armed daVinci surgical robot in the Issac gym simulator \cite{Liang2018GPU}.}
    \label{fig:init_setup}
    \vspace{-12pt}
\end{figure}

\subsection{DeformerNet  Details}
As shown in Fig.~\ref{fig:DeformerNet}, DeformerNet consists of two stages: feature vector extraction and defomation control inference. In the first stage, we perform convolution on 3D point clouds to extract feature vectors representing the states of the object shapes. This stage takes two point clouds as the inputs: one of the current object shape and one of the goal object shape. The output of this stage is two 256-dimension feature vectors. 

We then subtract the two feature vectors one from another and feed this to the second stage. The deformation control inference stage takes this 256-dimension \textit{differential feature vector} and passes it through a series of fully-connected layers (128, 64, and 32 neural units, respectively). The fully-connected output layer produces the 3D manipulation point displacement. Note that this is also equivalent to the robot’s end-effector Cartesian position displacement since the robot directly controls the position of the manipulation point. We use an ReLU activation function and batch normalization for all convolutional and fully-connected layers except for the output layer.

We use the standard mean squared error loss function for training our DNN. We adopt the Adam optimizer and a decaying learning rate which starts at $10^{-3}$ and decreases by 1/10 every 50 epochs. 

\subsection{Experiment Details}
Partial point clouds are generated and segmented out from the robot and background using the depth camera available inside the Issac gym environment. We sample 2048 points on each object point cloud using the Furthest Point Sampling method from \cite{Qi2017PointNet}. For the Keypoint Detection Heuristic method, we use 200 keypoints on each point cloud. The physical property of the object used in the experiment is: Young modulus = 1000 Pa, Poisson = 0.3.

\begin{figure*}[th!]
     \centering
     \begin{subfigure}[b]{\textwidth}
         \centering
         \includegraphics[width=1\textwidth]{figures/goal_vis_sample_0.png}
         \caption{Case 1 shape servo sequence}
     \end{subfigure}
     \hfill
     \begin{subfigure}[b]{\textwidth}
         \centering
         \includegraphics[width=1\textwidth]{figures/goal_vis_sample_2.png}
         \caption{Case 2 shape servo sequence}
     \end{subfigure}
     \hfill     
     \begin{subfigure}[b]{\textwidth}
         \centering
         \includegraphics[width=1\textwidth]{figures/goal_vis_sample_3.png}
         \caption{Case 3 shape servo sequence}
     \end{subfigure}
     \hfill
     \begin{subfigure}[b]{\textwidth}
         \centering
         \includegraphics[width=1\textwidth]{figures/goal_vis_sample_4.png}
         \caption{Case 4 shape servo sequence}
     \end{subfigure}
    \caption{Additional visualizations of the robot performing shape servoing to a variety of target shapes. The sparse red clouds visualize the target shapes of the object.}
    \label{fig:additional_vis}
\end{figure*}

\begin{figure*}[hb!]
    \centering
    \includegraphics[width=\linewidth]{figures/Chamfer.png}
    \caption{Chamfer distance between the current object point cloud and the goal object point cloud over time. From left to right: cases 1, 2, 3, \& 4 respectively.}
    \label{fig:chamfer_plots}
    \vspace{-12pt}
\end{figure*}
